# Supplementary material for: BOLA360: Near-optimal View and Bitrate Adaptation for 360-degree Video Streaming
Source: arXiv:2309.04023 source file (2024-10-01)
Supplement: Supplementary file 1 [file sec_appendix_baseline_algorithms.tex]

\section{More Details on Baseline Algorithms used in Experimental Evaluations i}
\label{app:baseline_algorithms}

\begin{algorithm}[!t]
\SetAlgoLined
\KwResult{$\textbf{a}_k$}
%  time split into chunks of $t_0$\;
%  if it is the first segment, initialize global variable $r_0 = 0$\;
 $r_{Max} = -\infty$ \tcp*[1]{store the reward of best action founded so far}
 $\textbf{a}_k = Null$ \tcp*[1]{keep the best action founded so far for chunk $k$}
%  $Time = \infty$\;
 
 \For {all possible tuples $\textbf{a} = [m^{(1)},m^{(2)},...,m^{(D)}]$}{
 $n: $ number of tiles inside \textbf{a} with positive bitrate\;
 $T: $ estimated-download-time($\textbf{a}$, $w_p(t)$)\;
%  $T' = \max[ T, b + n \delta - b_{max}]$\;
%  $T_{0}$ = $\lfloor T'/t_0 \rfloor t_0$\;
 
%  $R = \max[T_0 - b, 0]$\;
%  $t' = t + T_0$\;
%  $b' = b - T_0 + R + n \delta$\;
 $\forall i, \ v^{(i)} := v_{m^{(i)}}$\;
  $\forall i, \ a_{(i)} := 1$ if $m^{(i)} > 0$ else 0\;
 $r' = \gamma n \delta / T + \sum_{d=1}^{D}a_{(i)} (v^{(i)} p_{k, d}  - p_D\ . \ \beta) / T$\;
  \If{$r' > r_{Max}$}{
  $\textbf{a}_k = \textbf{a}$\;
  $r_{Max} =   r'$\;
 }
 }
%   after downloading \textbf{m}, update $r_0$\;
 \caption{\ddpON$(k, w_p(t), t, b)$}
 \label{alg:online_DP}
\end{algorithm}

\subsection{\ddpON: A Naive Online Algorithm with Prediction of Bandwidth}
\rev{Make sure to revise this section if you decide to remove previous section (optimal offline algorithm). You can mention this algorithm as a greedy algorithm} For online algorithms, calculating the download time is not possible at the moment of decision time since the bandwidth capacity is unknown. Let $w(t)$ be the actual bandwidth capacity at time $t$ and $w_p(t)$ be a prediction for bandwidth capacity at time $t$. Then, one can modify Algorithm~\ref{alg:opt_off} to an online algorithm, \ddpON, as described in Algorithm \ref{alg:online_DP}. \ddpON follows the same approach as Algorithm \ref{alg:opt_off} with some adjustments. The buffer level $b$ and time $t$ are given in Algorithm~\ref{alg:online_DP}. Based on these inputs and assuming that the predicted value for the bandwidth capacity is accurate, the best action is taken. The achieved QoE is updated based on the action taken and the actual download time.
More precisely, \ddpON estimates the download time of any possible action and heuristically selects the action that maximizes the QoE without any knowledge of the future. In an ideal case, the perfect prediction of bandwidth capacity can help this algorithm to work close to the optimal solution since its input is similar to the one for the offline algorithm. However, the performance of this algorithm degrades as the quality of the predictions decreases. \ddpON evaluates every possible action $\textbf{a}$ and the reward collected by taking this action in Line 8. Variables $\textbf{a}_{k}$ and $r_{\max}$ keep the best action found and its reward found so far. During our experiments, we calculate the average bandwidth for the past few seconds and use this value as the prediction of bandwidth, $w_p(t)$.

\subsection{\naive: A Naive Uniform Algorithm for Top Probable Tiles}

Another possible alternative for designing an online algorithm is based on the head position probability value of each tile. The \naive algorithm evenly distributes the bandwidth among $X$ highest probable tiles inside \AF. Let $[p_1, p_2, ..., p_D]$ be the head position probability values in an descending order, i.e., if $i < j$, then $p_i \leq p_j$. The \naive algorithm distributes the bandwidth capacity among top $X$ tiles with the highest probability, $\{i | p_X \leq p_i \}$, and downloads the same bitrate for all of these $X$ tiles and nothing for the rest. The algorithm is designed to select the highest possible bitrate in a way that rebuffering is expected to be zero. To this end, a chunk's download time is selected to be shorter than its playback time, which is constant $\delta$.
A key challenge is that the actual bandwidth capacity for the download time duration is unknown to the online algorithms. The \naive algorithm calculates the average bandwidth for the past few seconds and uses this value as the prediction of bandwidth to select the bitrates. The performance of the \naive algorithm depends on the bandwidth capacity's accuracy and the head position probability distribution. The pseudocode of the \naive algorithm is listed as Algorithm~\ref{alg:Naive}. We tested multiple values of $X$ between 1 to D to select the best \naive algorithm; We find that \naiveX{D} performs better among them. So we used \naiveX{D} in our empirical evaluations in Section \ref{sec:exp}.

\begin{algorithm}[!t]
\SetAlgoLined
% \KwResult{$r$}
% \\
 $p_{min} = $ probability of $X^{st}$ highest probable tile\\
 $r = \max \bigg\{m \ \bigg| \ m \in [1, 2, ..., M] ,\quad X S_m \leq \delta \  . \ w_p(t) \bigg\}$\\
 
 \For {tile $d \in [1, 2, ..., D]$}{
 \If{$p_{min} \leq p_{k,d}$}{
   select bitrate index $r$ for tile $d$ of chunk $k$\;
 }
 \Else{
  download nothing for tile $d$ of chunk $k$\;
 }
 
 }
%   after downloading \textbf{m}, update $r_0$\;
 \caption{\naive$(k)$}
 \label{alg:Naive}
\end{algorithm}

\subsection{\VAts: Bitrate Selection based on Probabilities as Weights}
The third comparison algorithm is \VAts, which is proposed in~\cite{ozcinar2017viewport}. The \VAts algorithm selects bitrate $\alpha w(t) \omega_d$ for tile $d$ such that $\alpha$ is a constant and $\omega_d$ is a weight of tile d among all tiles. In our experiments, we select the head direction probabilities as weight vectors and $\alpha = 1$. Since possible bitrates are discrete values, the bitrate selected for tile $d$ of chunk $k$ with head direction probability $p_{k, d}$ is rounded to the closest possible bitrate to the set of available bitrates.
% \begin{equation}
% \label{eq:VA360}
%     m^{(d)} = \arg\min_{m_i} |p_{k, d} w_p(t) - m_i |,
% \end{equation}
The intuition behind this algorithm is that the fraction of bandwidth allocated to each tile is proportional to the probability of the tile being inside \AF. Similar to other naive algorithms that take action based on the current bandwidth capacity value, the performance of this algorithm directly depends on the difference between the current bandwidth value and the average bandwidth during the download time.

\subsection{\PDash}
The fourth comparison algorithm is \PDash and proposed by Xie et al. ~\cite{xie2017360probdash}. The primary objective of this study is to distribute the available bitrates among different tiles in order to maximize the QoE. Unlike \algName, which independently selects the bitrates for each tile, \PDash determines the aggregate bitrates for all tiles within a chunk before distributing them across the individual tiles. To establish the aggregate bitrates for a chunk, \PDash focuses on maintaining the buffer level at a predetermined target level ($Q_{target}$). 
% Therefore, if $w_p(t)$ shows the estimated bandwidth capacity during download time, $Q(t)$ and $Q(t')$ show the buffer level before and after downloading a new segment with aggregate bitrate $B$, then we have:
% \begin{equation*}
%     Q(t') =  Q(t) - \frac{B \delta}{w_p(t)} + D \delta,
% \end{equation*}
% by setting $Q(t')$ equals to $Q_{target}$ we get:
% \begin{equation*}
%     B = \frac{w_p(t)}{\delta}(Q(t) - Q_{target} + D\delta).
% \end{equation*}
% In the next step, \PDash splits $B$ among all $D$ tiles in a way to maximize the QoE. Also, \PDash fetch at least the lowest available bitrate for each tile.

\subsection{\SalVR}
The final algorithm under consideration is \SalVR, as proposed in the publication by Wang et al.~\cite{wang2022salientvr}. In \SalVR, the estimated bandwidth and buffer level are utilized to determine the highest possible bitrates such that the download time for a new chunk (including all tiles) does not exceed the length of the buffered video. Specifically, \SalVR employs an algorithmic parameter, denoted by $Q_{thr}$, such that the estimated download time for the new chunk takes at most $Q_{avl}(t) - Q_{thr}$ (while downloading at least the lowest bitrate under any condition). Here, $Q_{avl}(t)$ represents the length of the buffered video at time $t$. Note that $Q_{avl}(t)$ is not necessarily equal to $Q(t)$, as $Q(t)$ may comprise multiple tiles of a single chunk. In a special case where the ABR algorithm downloads a segment for each tile, $Q_{avl}(t)$ is equivalent to $Q(t) / D$. By constraining the download time of the chunk to be no longer than $Q_{avl}(t) - Q_{thr}$ and utilizing the estimated bandwidth capacity $w_p(t)$, \SalVR selects an aggregate bitrate of $B_{max}(t) = w_p(t) \times (Q_{avl}(t) - Q_{thr}) / \delta$. Subsequently, \SalVR allocates the selected aggregate bitrate among the tiles such that the fraction of $B_{max}(t)$ assigned to tile $d$ corresponds to its probability, $p_{k, d}$.
