# Supplementary material for: BOLA360: Near-optimal View and Bitrate Adaptation for 360-degree Video Streaming
Source: arXiv:2309.04023 source file (2024-10-01)
Supplement: Supplementary file 2 [file sec_appendix_heursitics.tex]

\section{More Detail on the bitrate selection of \hrPL, \hrPA, and \hrREP}
\label{app:heuristics}

\subsection{\hrPL}
We extend the idea of \hrPL presented in \cite{spiteri2019theory} to generate \hrPL in order to reduce the oscillation and reaction time of \algName. The high level idea is to virtually increase the buffer level during start or seek time. Specifically, \hrPL uses the estimated bandwidth and multiply it by $50\%$ to achieve a safe expected bandwidth. Therefore, with a high chance the actual average bandwidth during downloading of a segment would be higher than the safe expected bandwidth. Given that, in order to avoid rebuffering, the size of new downloading chunk (including all tiles) should be less than $Q_{avl}(t) w_p(t) / 2$. In this equation, $Q_{avl}(t)$ shows the length of buffered video at time $t$. \hrPL virtually inserts proportional number of segments into the buffer such that the size of new downloading chunk does not exceed $Q_{avl}(t) w_p(t) / 2$.

\subsection{\hrPA}

The values of tile probabilities directly impact the decision-making process of \algName and this impact is not linear due to terms like $\gamma \delta$ and $Q(t_k)$ in Equation \ref{eq:alg_maximization}. It means that the actual values of probabilities affect the bitrates, not their relative values.  In addition, low probability values do not always indicate that the tile has a low chance of being watched. For example, in cases where the number of tiles is large, the probability value of each tile is small, resulting in \algName selecting low bitrates, irrespective of the network's capacity.
% The actual values of predicted head position probabilities directly impact the decision-making process of \algName. When these values are low, \algName tends to select low bitrates. However, low probability values do not always indicate that the tile has a low chance of being watched. For example, in cases where the number of tiles is large, the probability value of each tile is small, resulting in \algName selecting low bitrates, irrespective of the network's capacity.

To address this issue and enhance the practical performance of \algName in terms of rendered bitrates, we introduce \texttt{BOLA360-PA}. This heuristic approach adjusts the probability values by multiplying them by a selected value $\mathcal{F}_p$. This adjustment maintains the relative ratio of probabilities while increasing their actual value of probabilities. To prevent rebuffering, \hrPA estimates the network throughput and multiplies it by $0.5$ to determine a safe network throughput for the next download. Similar to the approach taken for \hrPL, \hrPA calculates the upper bound on the aggregate size of segments for the next download. It then selects the highest value for $\mathcal{F}_p$ that ensures the aggregate size of selected segments is smaller than the calculated upper bound.

\subsection{\hrREP}
One of the primary limitations of the \algName algorithm is its inability to modify previously downloaded segments. Specifically, \algName must make decisions about future segments, and it cannot replace higher bitrate segments with previously downloaded, lower quality ones. If the bandwidth capacity experiences a short-term decrease, \algName adjusts the download bitrates to match the new bandwidth capacity by switching to lower bitrates. When the bandwidth increases again, \algName may have already downloaded several segments with low bitrates, and it cannot replace them with higher quality ones, even if the buffer level and bandwidth capacity are high. Consequently, \algName cannot utilize the entire bandwidth opportunity to optimize QoE. This challenge is addressed by \hrREP.

\hrREP is an enhanced version of \algName that optimizes video streaming by intelligently adjusting previously downloaded segments. It evaluates whether to prioritize downloading segments for the next chunk or improving the quality of existing ones based on the length of video available in the buffer. If the available video in the buffer falls below a danger threshold of $2 \delta$, \hrREP downloads segments for the next chunk. Conversely, if the buffer surpasses the danger threshold, it replaces lower-quality segments with higher bitrates. To identify the segments for replacement, \hrREP identifies chunks where there is at least two levels difference between the downloaded bitrate and the bitrate \algName would currently select based on buffer level. By addressing these limitations, \hrREP enhances the overall streaming experience and improves user satisfaction.

% \hrREP is a variant of \algName that allows for modification of previously downloaded segments. Specifically, \hrREP determines whether it is better to download segments for the next chunk or to improve the quality of previously downloaded segments, based on the length of video available in the buffer. Specifically, \hrREP considers a danger-threshold equals to $2 \delta$, and downloads segments for the next chunk if the length of available video in buffer, $Q_{avl}(t)$ is less than danger-threshold. If $Q_{avl}(t)$ is over danger-threshold, then \hrREP replace a higher bitrates for previously downloaded segments; If the decision is to download segments for the next chunk, \hrREP selects the bitrates according to the decision of \algName. In the case of replacement, \hrREP identifies chunks where there is at least a two-level difference between the bitrate level downloaded for tiles of that chunk and the bitrates that \algName would select at the current time with current buffer level. \hrREP then downloads and replaces the new segments for those low-quality tiles. If no low-quality tiles are detected, \hrREP follows downloading segments for the next chunk as usual. Overall, \hrREP addresses the limitations of \algName and improves the quality of experience for users.
