# Supplementary material for: BOLA360: Near-optimal View and Bitrate Adaptation for 360-degree Video Streaming
Source: arXiv:2309.04023 source file (2024-10-01)
Supplement: Supplementary file 3 [file sec_appendix.tex]

%%
%% If your work has an appendix, this is the place to put it.
\appendix

 \onecolumn

% \section{Proof of Theorem \ref{thm:buffer_size} }
\section{More Detail on the Performance of \algName}
\label{app:buff_proof}
\begin{remark}
    Theorem \ref{thm:buffer_size} gives an upper bound for the buffer level used by \algName as a function of problem parameters and algorithm parameter $V$. The buffer usage of \algName grows linearly with the growth of $V$. Buffer level usage is an upper bound for the playback delay of the video. Based on this theorem, one can target lower playback delay decreasing the value of $V$.
\end{remark}
We prove this theorem by induction. The base case is $Q(t_1) = 0 \leq V (v_M + \gamma \delta ) + D$ that satisfies the statement of the theorem. Two cases are possible for value of $Q(t_k)$:
\begin{itemize}
    \item \textit{Case 1}: $Q(t_k) \leq V (v_M + \gamma \delta )$: in this case, the buffer level at time $t_{k+1}$ does not exceeds $Q(t_k) + D \leq V (v_M + \gamma \delta ) + D.$
    \item \textit{Case 2}: $V (v_M + \gamma \delta ) < Q(t_k) < V (v_M + \gamma \delta  ) + D$: In this case, the action at time $t_k$ is to download nothing for any tiles. Hence $Q(t_{k+1}) \leq Q(t_k)$.
\end{itemize}

Now, we proceed to analyze the QoE performance of \algName. With large $K$, the \tABR problem with rate stability constraint \cite{neely2010stochastic} is equivalent to the relaxed version of \tABR with limited buffer capacity, i.e.,

\begin{subequations}
\label{eq:rate-stability}
\begin{align*}
      Q(t) \leq Q_{max} \Rightarrow \lim_{K \to \infty} \frac{1}{K} \Exp \bigg\{\sum_{k = 1}^{K} \sum_{d=1}^{D} \sum_{m=1}^{M} a_{k, d, m} \delta \bigg\} \leq \lim_{K \to \infty} \frac{1}{K} \Exp \bigg\{\sum_{k = 1}^{K} n_k T_k \bigg\},
\end{align*}
\end{subequations}
% \begin{dmath}
%  \label{eq:rate-stability}
%       Q(t) \leq Q_{max} \Rightarrow \lim_{K \to \infty} \frac{1}{K} \Exp \bigg\{\sum_{k = 1}^{K} \sum_{d=1}^{D} \sum_{m=1}^{M} a_{k, d, m} \delta \bigg\} \leq \lim_{K \to \infty} \frac{1}{K} \Exp \bigg\{\sum_{k = 1}^{K} n_k T_k \bigg\},
%  \end{dmath}
 Any solution to \tABR with limited buffer capacity requires that the expected input rate into the buffer be less than or equal to the buffer's output rate. Otherwise, for the case of $K \to \infty$, the limited buffer capacity constraint does not hold. It is good to mention that any solution to \tABR with limited buffer capacity satisfies the rate stability constraint; however, the opposite statement is not necessarily true.

% We give a lower bound on QoE of \algName as a function of QoE of the optimal algorithm, $U_K^{*} + \gamma R_K^{*}$ for large videos, i.e., $K \to \infty$. Offline \tABR problem fits in the notation of optimization for renewal frames \cite{neely2012dynamic}. Precisely, by fixing renewal frame duration and letting the achieved QoE of downloading each tile represent penalty values in the notation of \cite{neely2012dynamic}, the offline \tABR problem can convert into an optimization problem over renewal frames. We first define the stationary algorithm for \tABR problem, and then we prove there exists a \textit{stationary algorithm} with expected QoE of $U_K^{*} + \gamma R_K^{*}$.

% In the following, we prove the existence of a \textit{stationary algorithm} with the optimal achievable expected QoE. The proof is done by leveraging the optimal solution to the optimization problem for renewal frames \cite{neely2012dynamic}. Then, we give a lower bound on QoE of \algName as a function of QoE of the optimal algorithm, $U_K^{*} + \gamma R_K^{*}$ for large videos, i.e., $K \to \infty$. 

\textbf{\textit{The stationary algorithm}}: In the context of \tABR problem, we define \textit{stationary algorithm} as an ABR algorithm that downloads a fixed set of bitrates for all segments. This algorithm uses a fixed set of bitrates, $\textbf{A}^{*}$, with size $D$ ($|\textbf{A}^{*} | = D$), and for each chunk $K$, it selects the bitrates such that the set of selected bitrates for all $D$ tiles are the same as the $\textbf{A}^{*}$. Note that the selected bitrate for each tile may vary over time depending on the head position probability values, while the set of bitrates selected for all tiles of the chunk remains fixed.

Offline \tABR problem fits in the notation of optimization for renewal frames \cite{neely2012dynamic}. Precisely, by fixing renewal frame duration and letting the achieved QoE of downloading each tile represent penalty values in the notation of \cite{neely2012dynamic}, the offline \tABR problem can convert into an optimization problem over renewal frames. Then, following Lemma 1 in \cite{neely2012dynamic}, we prove the existence of a stationary algorithm with QoE of $U_K^{*} + \gamma R_K^{*}$.

\begin{lemma}
\label{lem:stat_opt}
For the \tABR problem with a large video, i.e., $K \to \infty$, there exists a stationary algorithm that satisfies the rate stability constraint and achieves the expected QoE of $U_K^{*} + \gamma R_K^{*}$.
\end{lemma}
\begin{proof}
The proof of this lemma follows from Lemma 1 in \cite{neely2012dynamic} and continues with the approach taken for proof of Lemma 1 in \cite{spiteri2020bola}. Based on the definition of a stationary algorithm for the \tABR problem, the expected QoE of the stationary algorithm is the same as expected, achieving QoE on each slot, which satisfies the criteria of Lemma 1 in \cite{neely2012dynamic}.
\end{proof}

\section{Proof of Theorem \ref{thm:alg_perf}}
\label{app:proof}
% Proof of Equation \ref{eq:buffer}:
% $$\Delta Q(t_k) = Q(t_{k+1}) - Q(t_k) \leq D$$
% Cases:
% \begin{enumerate}
%     \item $Q(t_k) \leq V(v_M +\gamma \delta)$
%     \item $ V(v_M + \gamma \delta ) < Q(t_k) < V(v_M + \gamma \delta ) + D$
% \end{enumerate}
% Using induction. The base is $Q(t_1) = 0 \leq V(v_M + \gamma \delta ) + D$\\
% \textbf{Case1:} $Q(t_{k+1})  =  Q(t_k) + \Delta Q(t_k) \leq V(v_M + \gamma \delta ) + D$\\
% \textbf{Case2:} $V(v_M + \gamma \delta) - Q(t_k)  < 0$, therefore, no segment is going to be downloaded between $t_k$ and $t_{k+1}$. So, buffer does not increase.\\

Lets define the Lyapunov function $L(Q(t_k))$, and per-slot conditional Lyapunov drift $\Phi(t_k)$ as below
\begin{align*}
L(Q(t_k)) &= \frac{1}{2} Q^2(t_k),\\
\Phi(t_k) &= \Exp \{ \Delta\ L(Q(t_k))\  |\ Q(t_k) \} = \Exp \{L(Q(t_{k+1})) - L(Q(t_k))  | Q(t_k) \}.
\end{align*}

% $$L(Q(t_k)) = \frac{1}{2} Q^2(t_k),$$
% $$\Phi(t_k) = \Exp \{ \Delta L(Q(t_k))\} = \Exp \{L(Q(t_{k+1})) - L(Q(t_k)) \},$$
Depending on the buffer level, the value of $\Phi(t_k)$ can get derived using buffer level evolution described in Equation \eqref{eq:buffer_update}. Consider two cases: 1) $Q(t_k) \leq n_k T_k / \delta$ and, 2) $Q(t_k) > n_k T_k / \delta$. In the first case, the value of $\Phi(t_k)$ would be
\begin{align*}
    \Phi_1(t_k) = \Exp \{ \frac{1}{2} \big( \sum_{d=1}^D\sum_{m=1}^M a_{k, d, m} \big)^2  - \frac{1}{2} Q^2(t_k) | Q(t_k)\},
\end{align*}
 and in the second case the value of $\Phi(t_k)$ would be
\begin{align*}
    \Phi_2(t_k) = \Exp \big\{\frac{1}{2} \big(\sum_{d=1}^D\sum_{m=1}^M a_{k, d, m} - \frac{n_k T_k}{\delta} \big) ^2  -Q(t_k) \big( \frac{ n_k T_k}{\delta} - \sum_{d=1}^D\sum_{m=1}^M a_{k, d, m} \big)\big\} | Q(t_k) \bigg\}.
\end{align*}

Therefore, there would be an upper bound for the value $\Phi(t_k)$ of as below
\begin{subequations}
\begin{align*}
    \Phi(t_k) & \leq  \max  \{  \Phi_1(t_k),  \Phi_2(t_k) \}\\
    & \leq  \Exp \bigg\{ \frac{n^2_k T_k^2 + \delta^2 (\sum_{d=1}^D\sum_{m=1}^M a_{k, d, m})^2}{2\delta^2} | Q(t_k) \bigg\}-  Q(t_k) \Exp\bigg\{ \frac{n_k T_k}{\delta}  - \sum_{d=1}^D\sum_{m=1}^M a_{k, d, m} \} | Q(t_k) \bigg\}\\
    & \leq  \frac{D \delta^2 + \Psi}{2\delta^2} - Q(t_k)\Exp\bigg\{\frac{n_k T_k}{\delta} -\sum_{d=1}^D\sum_{m=1}^M a_{k, d, m} \} | Q(t_k) \bigg\}.
\end{align*}
\end{subequations}

% \begin{subequations}
% \begin{align*}
%     \Phi(t_k) & \leq  \max  \{  \Phi_1(t_k),  \Phi_2(t_k) \}\\
%     & \leq  \Exp \bigg\{ \frac{n^2_k T_k^2 + \delta^2 (\sum_{d=1}^D\sum_{m=1}^M a_{k, d, m})^2}{2\delta^2} | Q(t_k) \bigg\}-  Q(t_k) \Exp\bigg\{ \frac{n_k T_k}{\delta}  - \sum_{d=1}^D\sum_{m=1}^M a_{k, d, m} \} | Q(t_k) \bigg\}\\
%     & \leq \Exp\bigg\{ \frac{D \delta^2 + n_k^2 T_k^2}{2\delta^2} | Q(t_k) \bigg\} - Q(t_k)\Exp\bigg\{\frac{n_k T_k }{\delta} -\sum_{d=1}^D\sum_{m=1}^M a_{k, d, m} \} | Q(t_k) \bigg\}\\
%     & =  \frac{D \delta^2 + \Psi}{2\delta^2} - Q(t_k)\Exp\bigg\{\frac{n_k T_k}{\delta} -\sum_{d=1}^D\sum_{m=1}^M a_{k, d, m} \} | Q(t_k) \bigg\}.
% \end{align*}
% \end{subequations}

Now, by subtracting $V\Exp\bigg\{ \sum_{d=1}^D \sum_{m=1}^M a_{k, d, m}(p_{k,d} v_m+\gamma \delta) | Q(t_k) \bigg\}$ from both side, we have
\begin{subequations}
\begin{align*}
     \Phi(t_k) & - V\Exp\bigg\{ \sum_{d=1}^D \sum_{m=1}^M a_{k, d, m}(p_{k,d} v_m+\gamma \delta) | Q(t_k) \bigg\}&\\
    & \leq  \frac{D \delta^2 + \Psi}{2\delta^2} - Q(t_k) \Exp\bigg\{ \frac{n_k T_k}{\delta} - \sum_{d=1}^D\sum_{m=1}^M a_{k, d, m} | Q(t_k) \bigg\} -  V \Exp \bigg\{\sum_{d=1}^D \sum_{m=1}^M a_{k, d, m}(p_{k,d} v_m+\gamma \delta) | Q(t_k)  \bigg\}.
\end{align*}
\end{subequations}

Let $w_{\texttt{avg}}$ denotes the average bandwidth capacity during downloading chunk $k$. Then the conditional expected download time for chunk $k$, $\Exp \{ T_k | Q(t_k) \} = \Exp \{ \frac{1}{w_{\texttt{avg}}} \sum_{d=1}^D\sum_{m=1}^M a_{k, d, m}S_m  | Q(t_k) \}$, can get minimized without requiring any knowledge of $w_{\texttt{avg}}$ as follows.
\begin{subequations}
\begin{align*}
     \Phi(t_k)& - V\Exp\bigg\{ \sum_{d=1}^D  \sum_{m=1}^M a_{k, d, m}(p_{k,d} v_m+\gamma \delta)| Q(t_k) \bigg\} &\\
    & \leq  \frac{D \delta^2 + \Psi}{2\delta^2} - Q(t_k) \Exp\bigg\{ \frac{n_k T_k}{\delta} - \sum_{d=1}^D\sum_{m=1}^M a_{k, d, m}| Q(t_k) \bigg\} -V(U_K^* + \gamma R_K^*) \Exp \{ T_{k} | Q(t_k)\}.
\end{align*}
\end{subequations}

% \begin{subequations}
% \begin{align*}
%      \Phi(t_k)& - V\Exp\bigg\{ \sum_{d=1}^D  \sum_{m=1}^M a_{k, d, m}(p_{k,d} v_m+\gamma \delta)| Q(t_k) \bigg\} &\\
%     & \leq  \frac{D \delta^2 + \Psi}{2\delta^2} - Q(t_k) \Exp\bigg\{ \frac{n_k T_k}{\delta} - \sum_{d=1}^D\sum_{m=1}^M a_{k, d, m}| Q(t_k) \bigg\} -V \Exp \big\{ \sum_{d=1}^D \sum_{m=1}^M a_{k, d, m}^{*}(v_m+\gamma \delta) | Q(t_k) \big\} \bigg\}\\
%     & \leq  \frac{D \delta^2 + \Psi}{2\delta^2} - Q(t_k) \Exp\bigg\{ \frac{n_k T_k}{\delta} - \sum_{d=1}^D\sum_{m=1}^M a_{k, d, m}| Q(t_k) \bigg\} -V(U_K^* + \gamma R_K^*) \Exp \{ T_{k,d} | Q(t_k)\}.
% \end{align*}
% \end{subequations}
% $$\Rightarrow \Phi(t_k)- V\Exp\bigg\{ \sum_{d=1}^D  \sum_{m=1}^M a_{k, d, m}(p_{k,d} v_m+\gamma \delta - p_D\ . \ \beta) \bigg\}$$
% $$\leq  \frac{D \delta^2 + \Psi}{2\delta^2} - Q(t_k) \Exp\bigg\{ \frac{n_k T_k}{\delta} - \sum_{d=1}^D\sum_{m=1}^M a_{k, d, m} \bigg\}$$
% $$- V \Exp \bigg\{\sum_{d=1}^D \sum_{m=1}^M a_{k, d, m}^{*}(v_m+\gamma \delta - p_D\ . \ \beta)  \bigg\}$$
% $$\leq  \frac{D \delta^2 + \Psi}{2\delta^2} - Q(t_k) \Exp\bigg\{ \frac{n_k T_k}{\delta} - \sum_{d=1}^D\sum_{m=1}^M a_{k, d, m} \bigg\}$$
% $$- V(U^* + \gamma R^*) \Exp \{ T_{k,d} | Q(t_k)\},$$
The above equation holds since the decision of \algName at time $t_k$ is a solution of maximization equation detailed in Equation \eqref{eq:alg_act} 
% and 
% $$\Exp \big\{ \sum_{d=1}^D \sum_{m=1}^M a_{k, d, m}^{*}(v_m+\gamma \delta)|Q(t_k)\big\} \leq \Exp \big\{ \sum_{d=1}^D \sum_{m=1}^M a_{k, d, m}(v_m+\gamma \delta)|Q(t_k)\big\}.$$
Then, we have
\begin{subequations}
\begin{align*}
     \Phi(t_k)& - V\Exp\bigg\{ \sum_{d=1}^D  \sum_{m=1}^M a_{k, d, m}(p_{k,d} v_m+\gamma \delta)| Q(t_k) \bigg\} \\
    & \leq  \frac{D \delta^2 + \Psi}{2\delta^2} - Q(t_k) \bigg( \frac{\Exp{\{n_k\}}}{\delta} - \frac{\Exp \{ \sum_{d=1}^D\sum_{m=1}^M a^{*}_{k, d, m} \}}{\Exp\{T^{*}_k\}} \bigg)\Exp\{T_k \} -  V(U_K^* + \gamma R_K^*) \Exp \{ T_{k}\},
\end{align*}
\end{subequations}
%  $$\leq  \frac{D \delta^2 + \Psi}{2\delta^2} - Q(t_k) \bigg( \frac{\Exp{\{n_k\}}}{\delta} - \frac{\Exp \{ \sum_{d=1}^D\sum_{m=1}^M a^{*}_{d,m} \}}{\Exp\{T^{*}_k\}} \bigg)\Exp\{T_k \}$$
% $$- V(U^* + \gamma R^*) \Exp \{ T_{k,d}\},$$ 
where $a^{*}_{k, d, m}$ is the action of stationary algorithm for tile $d$ and bitrate index $m$ of chunk $k$ which satisfies the rate stability constraint \eqref{eq:rate-stability}. $T^{*}_k$ shows the length of download time for chunk $k$ while the stationary algorithm is taking action. Based on rate stability constraint \eqref{eq:rate-stability}, the second term in equation above is always negative, so
\begin{align*}
     \Phi(t_k)- V\Exp\bigg\{ \sum_{d=1}^D  \sum_{m=1}^M a_{k, d, m}(p_{k,d} v_m+\gamma \delta)| Q(t_k) \bigg\} \leq  \frac{D \delta^2 + \Psi}{2\delta^2} - V(U_K^* + \gamma R_K^*) \Exp \{ T_{k}\}.
\end{align*}

% \begin{multline*}
%      \Phi(t_k)- V\Exp\bigg\{ \sum_{d=1}^D  \sum_{m=1}^M a_{k, d, m}(p_{k,d} v_m+\gamma \delta)| Q(t_k) \bigg\} \leq  \frac{D \delta^2 + \Psi}{2\delta^2} - V(U_K^* + \gamma R_K^*) \Exp \{ T_{k,d}\}.
% \end{multline*}
% $$\Rightarrow \Phi(t_k)- V\Exp\bigg\{ \sum_{d=1}^D  \sum_{m=1}^M a_{k, d, m}(p_{k,d} v_m+\gamma \delta - p_D\ . \ \beta) \bigg\}$$
% $$\leq  \frac{D \delta^2 + \Psi}{2\delta^2} - V(U^* + \gamma R^*) \Exp \{ T_{k,d}\},$$
By taking the sum over $k \in \{1, 2, ..., K \}$ we have
\begin{subequations}
\begin{align*}
    \sum_{k=1}^K \Phi(t_k) & - \sum_{k=1}^K V\Exp\bigg\{ \sum_{d=1}^D  \sum_{m=1}^M a_{k, d, m}(p_{k,d} v_m+\gamma \delta )| Q(t_k) \bigg\} \leq \frac{D \delta^2 + \Psi}{2\delta^2}K  -  V(U_K^* + \gamma R_K^*) \Exp \{ T_{k}\} K.
\end{align*}
\end{subequations}

% \begin{subequations}
% \begin{align*}
%     \sum_{k=1}^K \Phi(t_k) & - \sum_{k=1}^K V\Exp\bigg\{ \sum_{d=1}^D  \sum_{m=1}^M a_{k, d, m}(p_{k,d} v_m+\gamma \delta )| Q(t_k) \bigg\}\\
%     &= \Exp\{ L(Q(t_K))\}  - V  \Exp\bigg\{\sum_{k=1}^K  \sum_{d=1}^D  \sum_{m=1}^M a_{k, d, m}(p_{k,d} v_m+\gamma \delta)| Q(t_k) \bigg\}\\
%     &\leq  \sum_{k=1}^K\frac{D \delta^2 + \Psi}{2\delta^2} - \sum_{k=1}^K V(U_K^* + \gamma R_K^*) \Exp \{T_{k,d}\}\\
%      &\leq \frac{D \delta^2 + \Psi}{2\delta^2}K  -  V(U_K^* + \gamma R_K^*) \Exp \{ T_{k,d}\} K.
% \end{align*}
% \end{subequations}

% $$\sum_{k=1}^K \Phi(t_k)- \sum_{k=1}^K V\Exp\bigg\{ \sum_{d=1}^D  \sum_{m=1}^M a_{k, d, m}(p_{k,d} v_m+\gamma \delta - p_D\ . \ \beta) \bigg\}$$
% $$= \Exp\{ L(Q(t_K))\} - V  \Exp\bigg\{\sum_{k=1}^K  \sum_{d=1}^D  \sum_{m=1}^M a_{k, d, m}(p_{k,d} v_m+\gamma \delta - p_D\ . \ \beta) \bigg\}$$
% $$\leq  \sum_{k=1}^K\frac{D \delta^2 + \Psi}{2\delta^2} - \sum_{k=1}^K V(U^* + \gamma R^*) \Exp \{T_{k,d}\},$$
% $$ \leq \frac{D \delta^2 + \Psi}{2\delta^2}K -  V(U^* + \gamma R^*) \Exp \{ T_{k,d}\} K. $$
By dividing all terms by $V \times K \times  \Exp\{T_{k} \}$, we get 
$$\frac{\Exp\{L(Q(t_K)) \}}{V K \Exp\{  T_{k} \}} - \texttt{OBJ}
\leq \frac{D \delta^2+\Psi}{2V\delta^2}\cdot \frac{1}{\Exp\{T_{k} \} } - (U_K^* + \gamma R_K^*).$$

Last, by taking the limit $K \to +\infty$ we get
$$(U_K^* + \gamma R_K^*) - \frac{D \delta^2 + \Psi}{2V\delta^2}\sigma \leq \texttt{OBJ}.$$

%optimal offline algorithm
% \input{sec_optimalOffline}

% baseline algorithms
% \input{sec_appendix_baseline_algorithms}

\section{Generating Probability Distributions for Head Position Probability Values Used in Section \ref{sec:Exp3} }
\label{app:prob_dist}
To investigate the impact of head position probability values on the performance of different algorithms, we use synthetic probabilities to simulate different real-world scenarios. Toward this, we generate the head position probability distributions based on three parameters $D_{\text{pos}}(k)$, $r_{\min}(k)$, and $\alpha_p(k)$. Parameter $D_{\text{pos}}(k)$ is the number of tiles with positive probability inside the head position probability values for chunk $k$, i.e., $D_{\text{pos}}(k) = |\{p_{k, d} | p_{k, d} > 0\}|$; $r_{\min}(k)$ represents the ratio between the minimum and maximum probabilities among probabilities of tiles for chunk $k$. Last, parameter $\alpha_p(k)$ determines the heterogeneity of the head position probability values for chunk $k$. We introduce several additional auxiliary notations to concretely define $\alpha_p(k)$. 
Let $p_{i}^{(L)}(k)$ be the probability of $i^{th}$ highest probable tile if there is a fixed step, $\Delta_p$, between the probability of each tile and the probability of the next tile in sorted order of probabilities. 
% In this case, the probability of $i^{th}$ probable tile would be $p_{i}^{(L)}(k) = p_{\max}(k) - \Delta_p (i - 1)$, where $p_{\max}(k)$ is constant for segment $k$.
We define the probability of $i^{th}$ highest probable tile as a function of $\alpha_p(k)$ as follows.
\begin{equation}
\label{eq:prob_profile_vals}
    p_{i}(k) =  \frac{1 - \alpha_p(k)} {D_{\text{pos}}(k)} + \alpha_p(k) p_{i}^{(L)}(k).
\end{equation}
 The higher values of $\alpha_p(k)$, the higher the accuracy of the prediction of \AF. Note that we have ${0 < D_{\text{pos}}(k) \leq D}$, $r_{\min}(k) \leq 1$ and $0 <\alpha_p(k) \leq 1$. With the above definition in Equation~\eqref{eq:prob_profile_vals}, $\alpha_p(k)$ determines the range of probabilities. In particular, $\alpha_p(k) = 0$ means the probability of all tiles are the same, i.e., $p_{i}(k) = 1 / D_{\text{pos}}(k)$. On the other hand, $\alpha_p(k) = 1$ spans a wide range of probabilities between the minimum and the maximum., representing heterogeneous values for the head position probability values. A justification for this model as a representative of real-world head direction prediction is that $(D - D_{\text{pos}})$ shows the number of tiles the \AF prediction model is confident that they will be out of \AF. On the other hand, $\alpha_p(k)$ shows how concentrated the \AF prediction model is. We use $r_{\min}(k) = 0.05$ for all distributions. Also, the details of the 12 probability distributions used in Section \ref{sec:Exp3} is listed in Table \ref{tbl:prob_profiles}.
\begin{table}[!t]
	\caption{The details of the probability distributions used in the experiment of Section~\ref{sec:Exp4}}
	% \vspace{-3mm}
	\label{tbl:prob_profiles}
 	\footnotesize
	\begin{center}
		\begin{tabular}[P]{|c|c|c|c|c|c|c|c|c|c|c|c|c|}
			\hline
			  \textbf{Probability profile index} &  \textbf{1}&  \textbf{2} &   \textbf{3} &   \textbf{4} &   \textbf{5} &   \textbf{6} &   \textbf{7} &   \textbf{8} &   \textbf{9} &   \textbf{10} &   \textbf{11} &   \textbf{12}\\
            \hline
            \textbf{$D_{\text{\text{pos}}}(k)$ }& 8 & 8 & 8 & 8 & 8 & 4 & 4 & 4 & 4 & 4 & 2 & 2\\
            \hline
            \textbf{$\alpha_p(k)$} & 0 & 0.25 & 0.5 & 0.75 & 1 & 0 & 0.25 & 0.5 & 0.75 & 1 & 0 & 0.5\\
            \hline

		\end{tabular}
	\end{center}
% 	\normalsize
\end{table}

% \begin{table}[!t]
% 	\caption{The details of the probability distributions used in the experiment of Section~\ref{sec:Exp4}}
% 	\vspace{-3mm}
% 	\label{tbl:prob_profiles}
%  	\footnotesize
% 	\begin{center}
% 		\begin{tabular}[P]{|c|c|c|}
% 			\hline
% 			\textbf{Distribution index} & $D_{\text{\text{pos}}}(k)$ & $\alpha_p(k)$ \\
% 			\hline
% 			\textbf{1} & 8 & 0 \\
% 			\hline
% 			\textbf{2} & 8& 0.25 \\
% 			\hline
% 			\textbf{3} & 8& 0.5 \\
% 			\hline
% 			\textbf{4} & 8& 0.75 \\
% 			\hline
% 			\textbf{5} & 8& 1 \\
% 			\hline
% 			\textbf{6} & 4& 0 \\
% 			\hline
% 			\textbf{7} & 4 & 0.25 \\
% 			\hline
% 			\textbf{8} & 4 & 0.5 \\
% 			\hline
% 			\textbf{9} & 4 & 0.75 \\
% 			\hline
% 			\textbf{10} & 4 & 10 \\
% 			\hline
% 			\textbf{11} & 2 & 0 \\
% 			\hline
% 			\textbf{12} & 2 & 0.5 \\
% 			\hline
% 		\end{tabular}
% 	\end{center}
% % 	\normalsize
% \end{table}

% heuristic improvements
% \input{sec_appendix_heursitics}

\section{Network Profiles Used In Section \ref{sec:exp} and \ref{sec:Exp3}}
\label{app:network_profiles}
The network profiles used in Section \ref{sec:exp} and \ref{sec:Exp3} are plotted in Figure \ref{fig:network_profiles}. The network profile index 15 shows 4G bandwidth traces published in \cite{bokani2016prehensive} and network profile 1-14 are from 4G/LTE bandwidth trace dataset \cite{IDLAB} collected by IDLAB \cite{ vanderHooft2016}.
\begin{figure}
    \centering
    \includegraphics[width=0.95\textwidth, height=1.2 \textwidth]{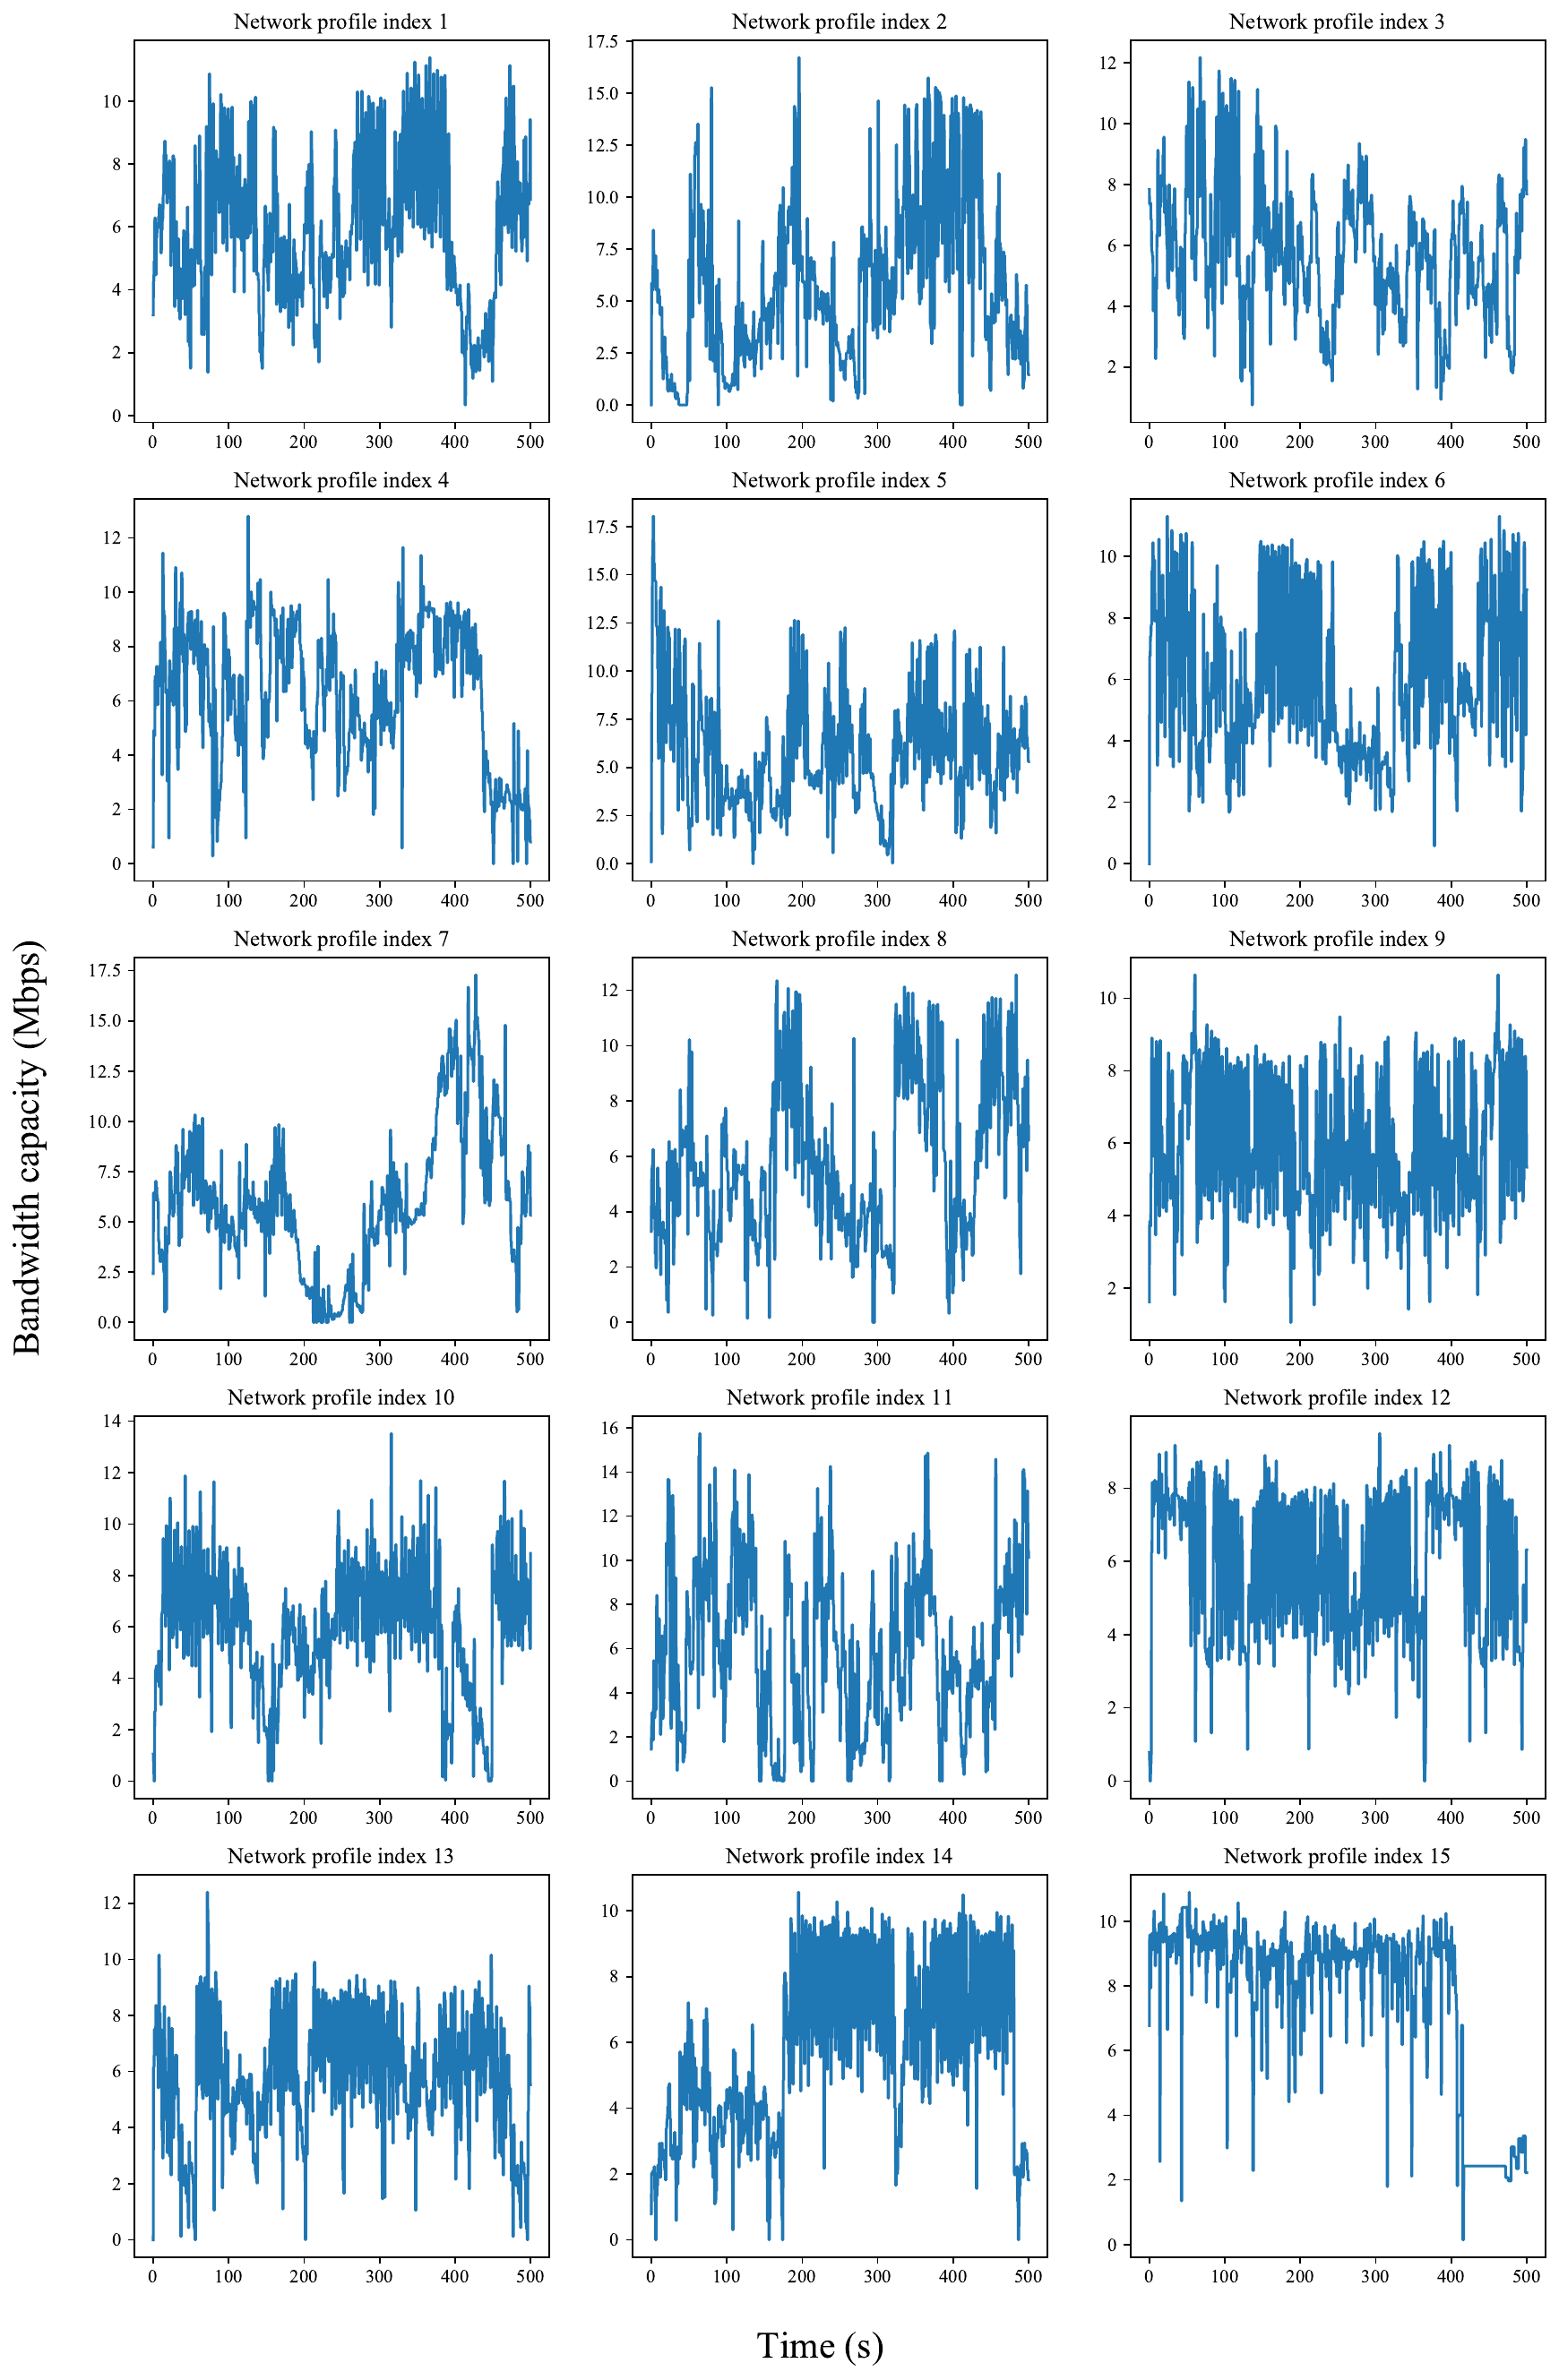}
    \caption{Fifteen network profiles used in experiments of Section \ref{sec:exp} and Section \ref{sec:Exp3}.}
    \label{fig:network_profiles}
\end{figure}
