# Supplementary material for: BOLA360: Near-optimal View and Bitrate Adaptation for 360-degree Video Streaming
Source: arXiv:2309.04023 source file (2024-10-01)
Supplement: Supplementary file 4 [file Details-of-additional-contribution.tex]

\documentclass[11pt,a4paper,sans]{article}


\usepackage{lipsum} 
\usepackage{subcaption}
\usepackage{natbib} 
\usepackage[scale=0.77]{geometry} 
\geometry{top=1in, bottom=1in}
%----------------------------------------------------------------------------------------
%	NAME AND CONTACT INFORMATION SECTION
%----------------------------------------------------------------------------------------
\usepackage{caption}
\usepackage{graphicx}
\usepackage{float}
\pagenumbering{gobble}
\usepackage{xspace}
\newcommand{\algName}{\texttt{BOLA360}\xspace}

\title{Explanation of Additional Contributions in the ACM TOMM Submission}


\begin{document}
\noindent  Dear Editor,\\

We are pleased to submit our manuscript titled "\algName: Near-optimal View and Bitrate Adaptation for 360-degree Video Streaming" for consideration in ACM Transactions on Multimedia Computing, Communications, and Applications (TOMM). This work builds upon our previous publication in the 2024 ACM Multimedia Systems (MMSys) Conference. However, due to the page limitations at MMSys, several key contributions could not be included in the camera-ready version.

The submitted TOMM version represents a comprehensive and significantly extended version of the paper, containing over 25\% new material. Below, we highlight additional contributions and other changes included in this submission:

% This manuscript builds upon our previous work, which was published in the 2024 ACM Multimedia Systems (MMSys) Conference. Due to the page limitations in the MMSys conference, several important contributions could not be included in the final camera-ready version. The submission to ACM Transactions on Multimedia Computing, Communications, and Applications (TOMM) includes a full and extended version of the work, with at least 25\% new material. Below, we detail the additional contributions that have been included in this TOMM version:

\begin{enumerate}
    \item \textbf{Entirely New Section and Algorithm – Optimal Offline Algorithm:}
    
        We have introduced an entirely new section (Section 4) that presents an optimal offline algorithm for the online bitrate control problem. Calculating the QoE of optimal offline algorithm is crucial for understanding the performance of online algorithms, as it allows us to quantify the gap between their QoE and the maximum achievable QoE. This section provides a thorough explanation of the optimal offline algorithm, along with proofs of its correctness, which were not part of the MMSys version.
         
     \item \textbf{Providing Proof of Theorem 5.2 (Main Theorem of the Paper):}
     
     In the MMSys version, only a sketch of the proof for Theorem 5.2, which asserts the optimality of BOLA360, was included. In the TOMM version, we have provided a complete and rigorous proof for this theorem. While the sketch offered a high-level overview, the complete proof adds significant value and is a crucial part of the contribution in this work.

    \item \textbf{New Evaluation Metric – Wasted Bandwidth:} 
    Wasted bandwidth is a key metric for assessing the efficiency of online ABR algorithms, particularly in the context of 360-degree video streaming. It measures how effectively the available bandwidth is utilized. Due to space constraints, we omitted the comparison of wasted bandwidth between BOLA360 and other ABR algorithms in the MMSys version. In the TOMM version, we used wasted bandwidth as an additional evaluation metric to compare BOLA360 with other ABR algorithms. This is a significant extension, and Figures 11 and 12, which present the wasted bandwidth results, are entirely new to this submission.

    


     \item \textbf{Updated Evaluation Metric – Normalized Quality of Experience (QoE):} 
     
     We have added a new  QoE metric that is obtained by normalizing it against the optimal offline algorithm. We believe that this metric makes the QoE comparisons more understandable and meaningful for readers. The new QoE metric is presented in Figures 7, 9, and 13.


    \item \textbf{Enhanced Reproducibility – Experimental Setup Details:} 
    
    The new version includes comprehensive details of the experimental setup, which were not fully presented in the MMSys paper. This includes additional information on the video sequences and head position probability distributions used in our evaluation, detailed in Tables 2, 3, and 4.

         
    \item \textbf{Clarification of the Paper Presentation:} 
    
    The presentation of several sections have been improved for better clarity and more detailed explanations. Notable extensions include Section 6.5, the final two paragraphs of Section 7, the full proof of Theorem 5.1 in Section 5.2, and minor revisions to the Introduction for better readability.

    \item \textbf{Expanded Related Work Section:} 
    
    Due to page constraints, we could not provide a comprehensive review of the related work in the MMSys paper. In this version, we have expanded the related work section to include the most recent advances in online 360-degree video streaming.

\end{enumerate}
    
These enhancements make the current version more complete and technically robust, meeting the journal’s requirement for 25\% new material. We believe these additions significantly contribute to the research community and improve the overall quality of the manuscript.\\

Thank you for considering our paper for publication in ACM TOMM.\\

\noindent Sincerely,\\
Ali Zeynali, and Co-authors\\
\noindent University of Massachusetts, Amherst
    


% This work is previously published in ACM Multimedia System (MMSys) Confrence on 2024. Due to pages limits of the MMSys confrence some part of contributions did not published in the camera ready version. The version we submitted to the ACM Transactions on Multimedia Computing, Communications includes the full version of the paper with additional technical contributions. We have listed the main contributions that firstly appeared in the version submitted to TOMM.

% \begin{enumerate}
%     \item \textbf{Optimal Offline Algorithm}. We have added an entire new section (Section 4 of the submitted version) providing an optimal offline algorithm for the online bitrate control problem. This section includes the detail of the optimal offline algorithm, and theorems regarding its proof of correctness.
%     \item \textbf{Proof of Theorem 5.2}. Theorem 5.2 is the main theorem of the paper stating the optimality of the BOLA360. In the version submitted to MMSys Confrence, only a sketch of the proof provided while the full proof of this theorem is presented in the TOMM version.
%     \item \textbf{Full details of experiment setup}. The new version includes the full details of the experiment setup, including some informations that did not appear in the MMSys version. This includes Table 2 and 3, 4 which provides detail of the video, and head position probability distributions used in experimental evaluation.
%     \item {\textbf{Providing Normalized QoE}.} In the MMSys version the absolute value of QoE of algorithms provided in the experimental evaluation section. That raised a concern about understaning of the quality of QoE when its absolute value was plotted. By providing the optimal offline algorithm in the new version, we revised the QoE values in the experimental section and replaced them by the normalized value to be more understandable for the users and they can compare it easily with the best algorithm (optimal offline algorithm). This impacted Figure 7, Figure 9, and Figure 13.
%     \item \textbf{New metric of evaluation}. We provided a wasted bandwidth as a additional metric of evaluation for comparing BOLA360 with other ABR algorithms. Figure 11 and Figure 12 are completely new for this submission.

%     \item \textbf{Extra details}. We also have extended additional details regarding the clearity of algorithms and methods presented in this paper. This includes Section 6.5, Final two paragraphs of section 7, full proof of theorem 5.1 in section 5.2, and minor changes in the introduction. 
    
% \end{enumerate}


\end{document}
